# Supplementary material for: Assessing Security and Performances of Consensus algorithms for Permissioned Blockchains
Source: arXiv:1805.03490 source file (2018-05-09)

p

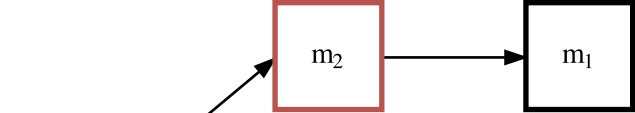

q

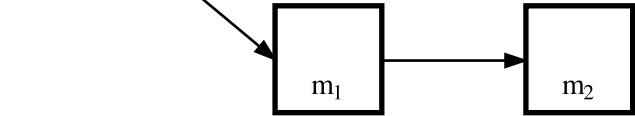

Supplement: Supplementary file 2 [file fi-proof2.pdf]
